# Supplementary material for: Assessing Privacy Risks from Feature Vector Reconstruction Attacks
Source: arXiv:2202.05760 source file (2022-02-11)
Supplement: Supplementary file 1 [file appendix.tex]

\section{Appendix}

\subsection{Ablation Results}

Here, we present ablation results across datasets, architectures, and
FVR methods. See Tables~\ref{tab:abl_web},~\ref{tab:abl_vgg}, and~\ref{tab:abl_scrub}.

\begin{table*}
  \centering
  \resizebox{0.99\textwidth}{!}{
\begin{tabular}{|c|c|rccc|cccr|} 
\hline
\multirow{3}{*}{\begin{tabular}[c]{@{}c@{}}\textbf{ Inversion }\\\textbf{Model }\end{tabular}} & \multirow{3}{*}{\begin{tabular}[c]{@{}c@{}}\textbf{ FVR}\\\textbf{Method }\end{tabular}} & \multicolumn{8}{c|}{\textbf{Test Models/Dataset}} \\ 
\cline{3-10}
 &  & \multicolumn{4}{c|}{Res50} & \multicolumn{4}{c|}{Efficient} \\ 
\cline{3-10}
 &  & \textit{WebFace} & \textit{VGGFace2} & \textit{Scrub} & \textit{LFW} & \textit{WebFace} & \textit{VGGFace2} & \textit{Scrub} & \textit{LFW} \\ 
\hline
\multirow{4}{*}{Res50} & NBNet & $18\%$ & $17\%$ & $6\%$ & $8\%$ & $10\%$ & $13\%$ & $7\%$ & $5\%$ \\
 & Vec2Face & $48\%$ & $14\%$ & $9\%$ & $2\%$ & $39\%$ & $11\%$ & $5\%$ & $3\%$ \\
 & Naive & $4\%$ & $8\%$ & $1\%$ & $4\%$ & $6\%$  & $9\%$ & $1\%$ & $2\%$ \\
  & Eigenfaces & $100\%$ & $100\%$ & $99\%$ & $99\%$ & $82\%$ & $60\%$ & $88\%$ & $82\%$ \\ 
\hline
\multirow{4}{*}{Efficient} & NBNet &  $4\%$ &  $13\%$&  $5\%$ & $6\%$ & $1\%$ & $9\%$ & $5\%$ & $3\%$ \\
 & Vec2Face & $33\%$ & $9\%$ & $3\%$ & $2\%$ & $42\%$ & $11\%$ & $3\%$ & $4\%$ \\
 & Naive & $5\%$ & $13\%$ & $0\%$ & $8\%$ & $5\%$ & $7\%$ & $3\%$ & $2\%$  \\
 & Eigenfaces & $81\%$ & $63\%$ & $88\%$ & $78\%$ & $99\%$ & $97\%$ & $96\%$ & $99\%$ \\
\hline
\end{tabular}
}
\caption{$tpr$ for $N=1000$, $K=25$ when FVR models are trained on the
  \texttt{WebFace} dataset.}
\label{tab:abl_web}
\end{table*}

\begin{table*}
  \centering
  \resizebox{0.99\textwidth}{!}{
\begin{tabular}{|c|c|rccc|cccr|} 
\hline
\multirow{3}{*}{\begin{tabular}[c]{@{}c@{}}\textbf{ Inversion }\\\textbf{Model }\end{tabular}} & \multirow{3}{*}{\begin{tabular}[c]{@{}c@{}}\textbf{ FVR}\\\textbf{Method }\end{tabular}} & \multicolumn{8}{c|}{\textbf{Test Models/Dataset}} \\ 
\cline{3-10}
 &  & \multicolumn{4}{c|}{Res50} & \multicolumn{4}{c|}{Efficient} \\ 
\cline{3-10}
 &  & \textit{WebFace} & \textit{VGGFace2} & \textit{Scrub} & \textit{LFW} & \textit{WebFace} & \textit{VGGFace2} & \textit{Scrub} & \textit{LFW} \\ 
\hline
\multirow{4}{*}{Res50} & NBNet & $6\%$ & $38\%$ & $3\%$ & $6\%$ & $8\%$ & $23\%$ & $5\%$ & $7\%$ \\
 & Vec2Face & $25\%$ & $29\%$ & $2\%$ & $3\%$ & $25\%$ & $26\%$ & $0\%$ & $2\%$ \\
 & Naive & $4\%$ & $12\%$ &  $3\%$ & $5\%$ & $5\%$ & $12\%$ & $5\%$ & $5\%$ \\
    & Eigenfaces & $100\%$ & $100\%$ & $99\%$ & $99\%$ & $82\%$ & $60\%$ & $88\%$ & $82\%$ \\ 
\hline
\multirow{4}{*}{Efficient} & NBNet & $5\%$ & $25\%$ & $4\%$ & $7\%$ & $4\%$& $17\%$ & $4\%$& $7\%$ \\
 & Vec2Face & $11\%$ & $25\%$ & $3\%$ & $3\%$ & $28\%$ & $31\%$ & $1\%$ & $1\%$ \\
 & Naive & $3\%$ & $11\%$ & $7\%$ & $12\%$ & $5\%$ & $10\%$ & $5\%$ & $11\%$ \\
   & Eigenfaces & $80\%$ & $63\%$ & $86\%$ & $76\%$ & $99\%$ & $97\%$ & $96\%$ & $99\%$ \\
\hline
\end{tabular}
}
\caption{$tpr$ for $N=1000$, $K=25$ when FVR models are trained on the
  \texttt{VGGFace2} dataset.}
\label{tab:abl_vgg}
\end{table*}

\begin{table*}
  \centering
  \resizebox{0.99\textwidth}{!}{
\begin{tabular}{|c|c|rccc|cccr|} 
\hline
\multirow{3}{*}{\begin{tabular}[c]{@{}c@{}}\textbf{ Inversion }\\\textbf{Model }\end{tabular}} & \multirow{3}{*}{\begin{tabular}[c]{@{}c@{}}\textbf{ FVR}\\\textbf{Method }\end{tabular}} & \multicolumn{8}{c|}{\textbf{Test Models/Dataset}} \\ 
\cline{3-10}
 &  & \multicolumn{4}{c|}{Res50} & \multicolumn{4}{c|}{Efficient} \\ 
\cline{3-10}
 &  & \textit{WebFace} & \textit{VGGFace2} & \textit{Scrub} & \textit{LFW} & \textit{WebFace} & \textit{VGGFace2} & \textit{Scrub} & \textit{LFW} \\ 
\hline
\multirow{4}{*}{Res50} & NBNet & $4\%$ & $11\%$ & $12\%$ & $3\%$ & $6\%$ & $11\%$ & $13\%$ & $6\%$ \\
 & Vec2Face & $33\%$ & $12\%$ & $30\%$ & $13\%$ & $20\%$ & $7\%$ & $36\%$ & $18\%$ \\
 & Naive & $6\%$ & $10\%$ & $2\%$ & $4\%$ & $4\%$ & $8\%$ & $6\%$ & $6\%$ \\
   & Eigenfaces & $100\%$ & $100\%$ & $98\%$ & $99\%$ & $82\%$ & $60\%$ & $88\%$ & $82\%$ \\ 
\hline
\multirow{4}{*}{Efficient} & NBNet & $3\%$ & $9\%$ & $3\%$ & $2\%$ & $4\%$ & $10\%$ & $4\%$ & $4\%$ \\
 & Vec2Face & $22\%$ & $11\%$ & $22\%$ & $7\%$ & $29\%$ & $10\%$ & $29\%$ & $13\%$ \\
 & Naive & $9\%$ & $8\%$ & $3\%$ & $1\%$ & $11\%$ & $12\%$ & $2\%$ & $12\%$ \\
 & Eigenfaces & $80\%$ & $63\%$ & $86\%$ & $76\%$ & $99\%$ & $97\%$ & $96\%$ & $99\%$ \\
\hline
\end{tabular}
}
\caption{$tpr$ for $N=1000$, $K=25$ when FVR models are trained on the
  \texttt{Scrub} dataset.}
\label{tab:abl_scrub}
\end{table*}

\subsection{Cost Analysis of FVR}

An interesting point of investigation, albeit one orthogonal to the
main goals of this paper, is assessing {\em real world cost} of
FVR attacks. FVR would be most devastating if successful in inverting
face embeddings from commercial facial recognition models like \texttt{Azure} and \texttt{Rekognition}, which
are widely used by numerous entities~\todo{CITE}. However, these models
require users to pay per query made to the model, meaning FVR attacks against
such models may prove costly. Thus, we perform a small study to
determine the cost and feasibility of inverting \texttt{Azure} and
\texttt{Rekognition}, using the FVR methods tested in this
paper. Below, we outline the assumptions in our study and our
findings.

\para{Assumptions and Attack Method.} We assume the attacker has black box access to
each of the commercial models with an unlimited number of queries. We
also assume the model return similarity scores quantifying the
difference between queried images and images enrolled in the reference
database. Finally, after the FVR model is trained, we assume the
attacker has access to a reference database of images enrolled in the
commercial system which they wish to invert.

The attacker conducts their attack as follows:
\begin{packed_enumerate}
  \item For the parametric methods, the attacker adds their entire training dataset to the
reference database for the commercial model. This is easily done,
since \texttt{Azure} and \texttt{Rekognition} allow users to create
and manage their own reference databases and allow paid users to
enroll tens of thousands of images. 
  \item Then, the attacker repeated queries the model during the
    training/optimization process. The model returns similarity
    score between the reconstructed images and the real enrolled
    images, which the attacker uses to guide their training. 
\end{packed_enumerate}
each query, the model returns a similarity score between the queried
image and a particular image in its enrolled reference database.

\para{Results.}  Table~\ref{tab:realworld} showcases our findings. The
cost for training parametric models is immense, as expected. However,
the Eigenfaces method could be conducted for a single image at a
baseline cost of \$200. 

\begin{table*}[h]
  \centering
  \resizebox{0.99\textwidth}{!}{
    \begin{tabular}{c|r|r|r} 
      \hline
      \textbf{FVR Method} & \# \textbf{Queries} & \multicolumn{1}{c|}{\textbf{Azure cost}} & \multicolumn{1}{c}{\textbf{AWS cost}}  \\ 
      \hline
      Eigenfaces (single image) &  200,000 & \$200 &  \$200 (queries) + \$0 (database) = \$200 \\
      Naive (model training) &  4,571,370 &  \$3,857 &  \$3,857 (queries) + \$42.76 (database) = \$3,900 \\
      NBNet (model training) &  38,010,960 &  \$6,181 & \$8,368 (queries) + \$175.80 (database) = \$8,544 \\
      Vec2Face (model training) &  15,000,000 &  \$4,800 & \$8,500 (queries) + \$83.75 (database) = \$8,583\\
      \hline
    \end{tabular}
  }
  \vspace{0.05cm}
  \caption{{\em Real-world cost of training a feature vector reconstruction model against Azure and AWS models. We assume the attacker trains the reconstruction model using the Webface dataset, which has 10,575 classes and 475,137 images. We assume each reconstruction method is trained/executed following the methodology in \S\ref{sec:method}.}}
\label{tab:realworld}
\end{table*}

\para{Discussion.} The results shown here represent the absolute
minimum baseline cost for FVR attacks against \texttt{Azure} and
\texttt{AWS}. In reality, the attacks would likely cost much
more, since if the commercial system will not return similarity scores
when query images are too dissimilar from enrolled images. This would
increase the number of attack queries needed. Finally, given the
high cost needed to conduct these attacks, it may be more
cost-effective for the attacker to consider other means of obtaining
information about enrolled images in a reference database, e.g. paying
off someone with access to the images.

\subsection{LPIPs as proxy for user study}

\todo{REWRITE}
Due to the high cost of conducting user studies, we investigate
whether a metric like $LPIPS$ could serve as a cheaper proxy. $LPIPS$ is measured by comparing $\tx$ and
the original image of $P$ that produced $v$ directly, to allow the most
accurate measurement. Although this comparison would be impossible in
a real-world scenario, we use it here as a baseline for each method's
overall visual fidelity to $P$. We measure $LPIPS$ similarity using $\tx$ generated from three
different datasets: \texttt{FaceScrub}, \texttt{VGGFace2}, and
\texttt{LFW}.

\para{Result: \texttt{NBNet} and \texttt{Eigenfaces} exhibit highest
  visual similarity.} As Figure~\ref{fig:visual1} demonstrates, \texttt{NBNet}
and \texttt{Eigenfaces} consistently have the highest $LPIPS$ scores
across all datasets. Even though the GAN-based nature of
\texttt{Vec2Face} produces more {\em realistic-looking} faces (see
Fig.~\ref{fig:all_reconstr}), it fails to capture more nuanced face
features, reducing the $LPIP$s score.

\emily{old text} While $LPIPS$ provides an important proxy for overall visual
similarity betweeen $\tx$ and $P$'s appearance, it is far from
complete. In fact, Figure~\ref{fig:visual2} shows that there is no direct correlation
between LPIPs score and feature space similarity (i.e. which determine
the set of top-K matches produced by a FR system).

\begin{figure}[b]
\centering
\begin{minipage}{.59\textwidth}
  \centering
  \includegraphics[width=.99\linewidth]{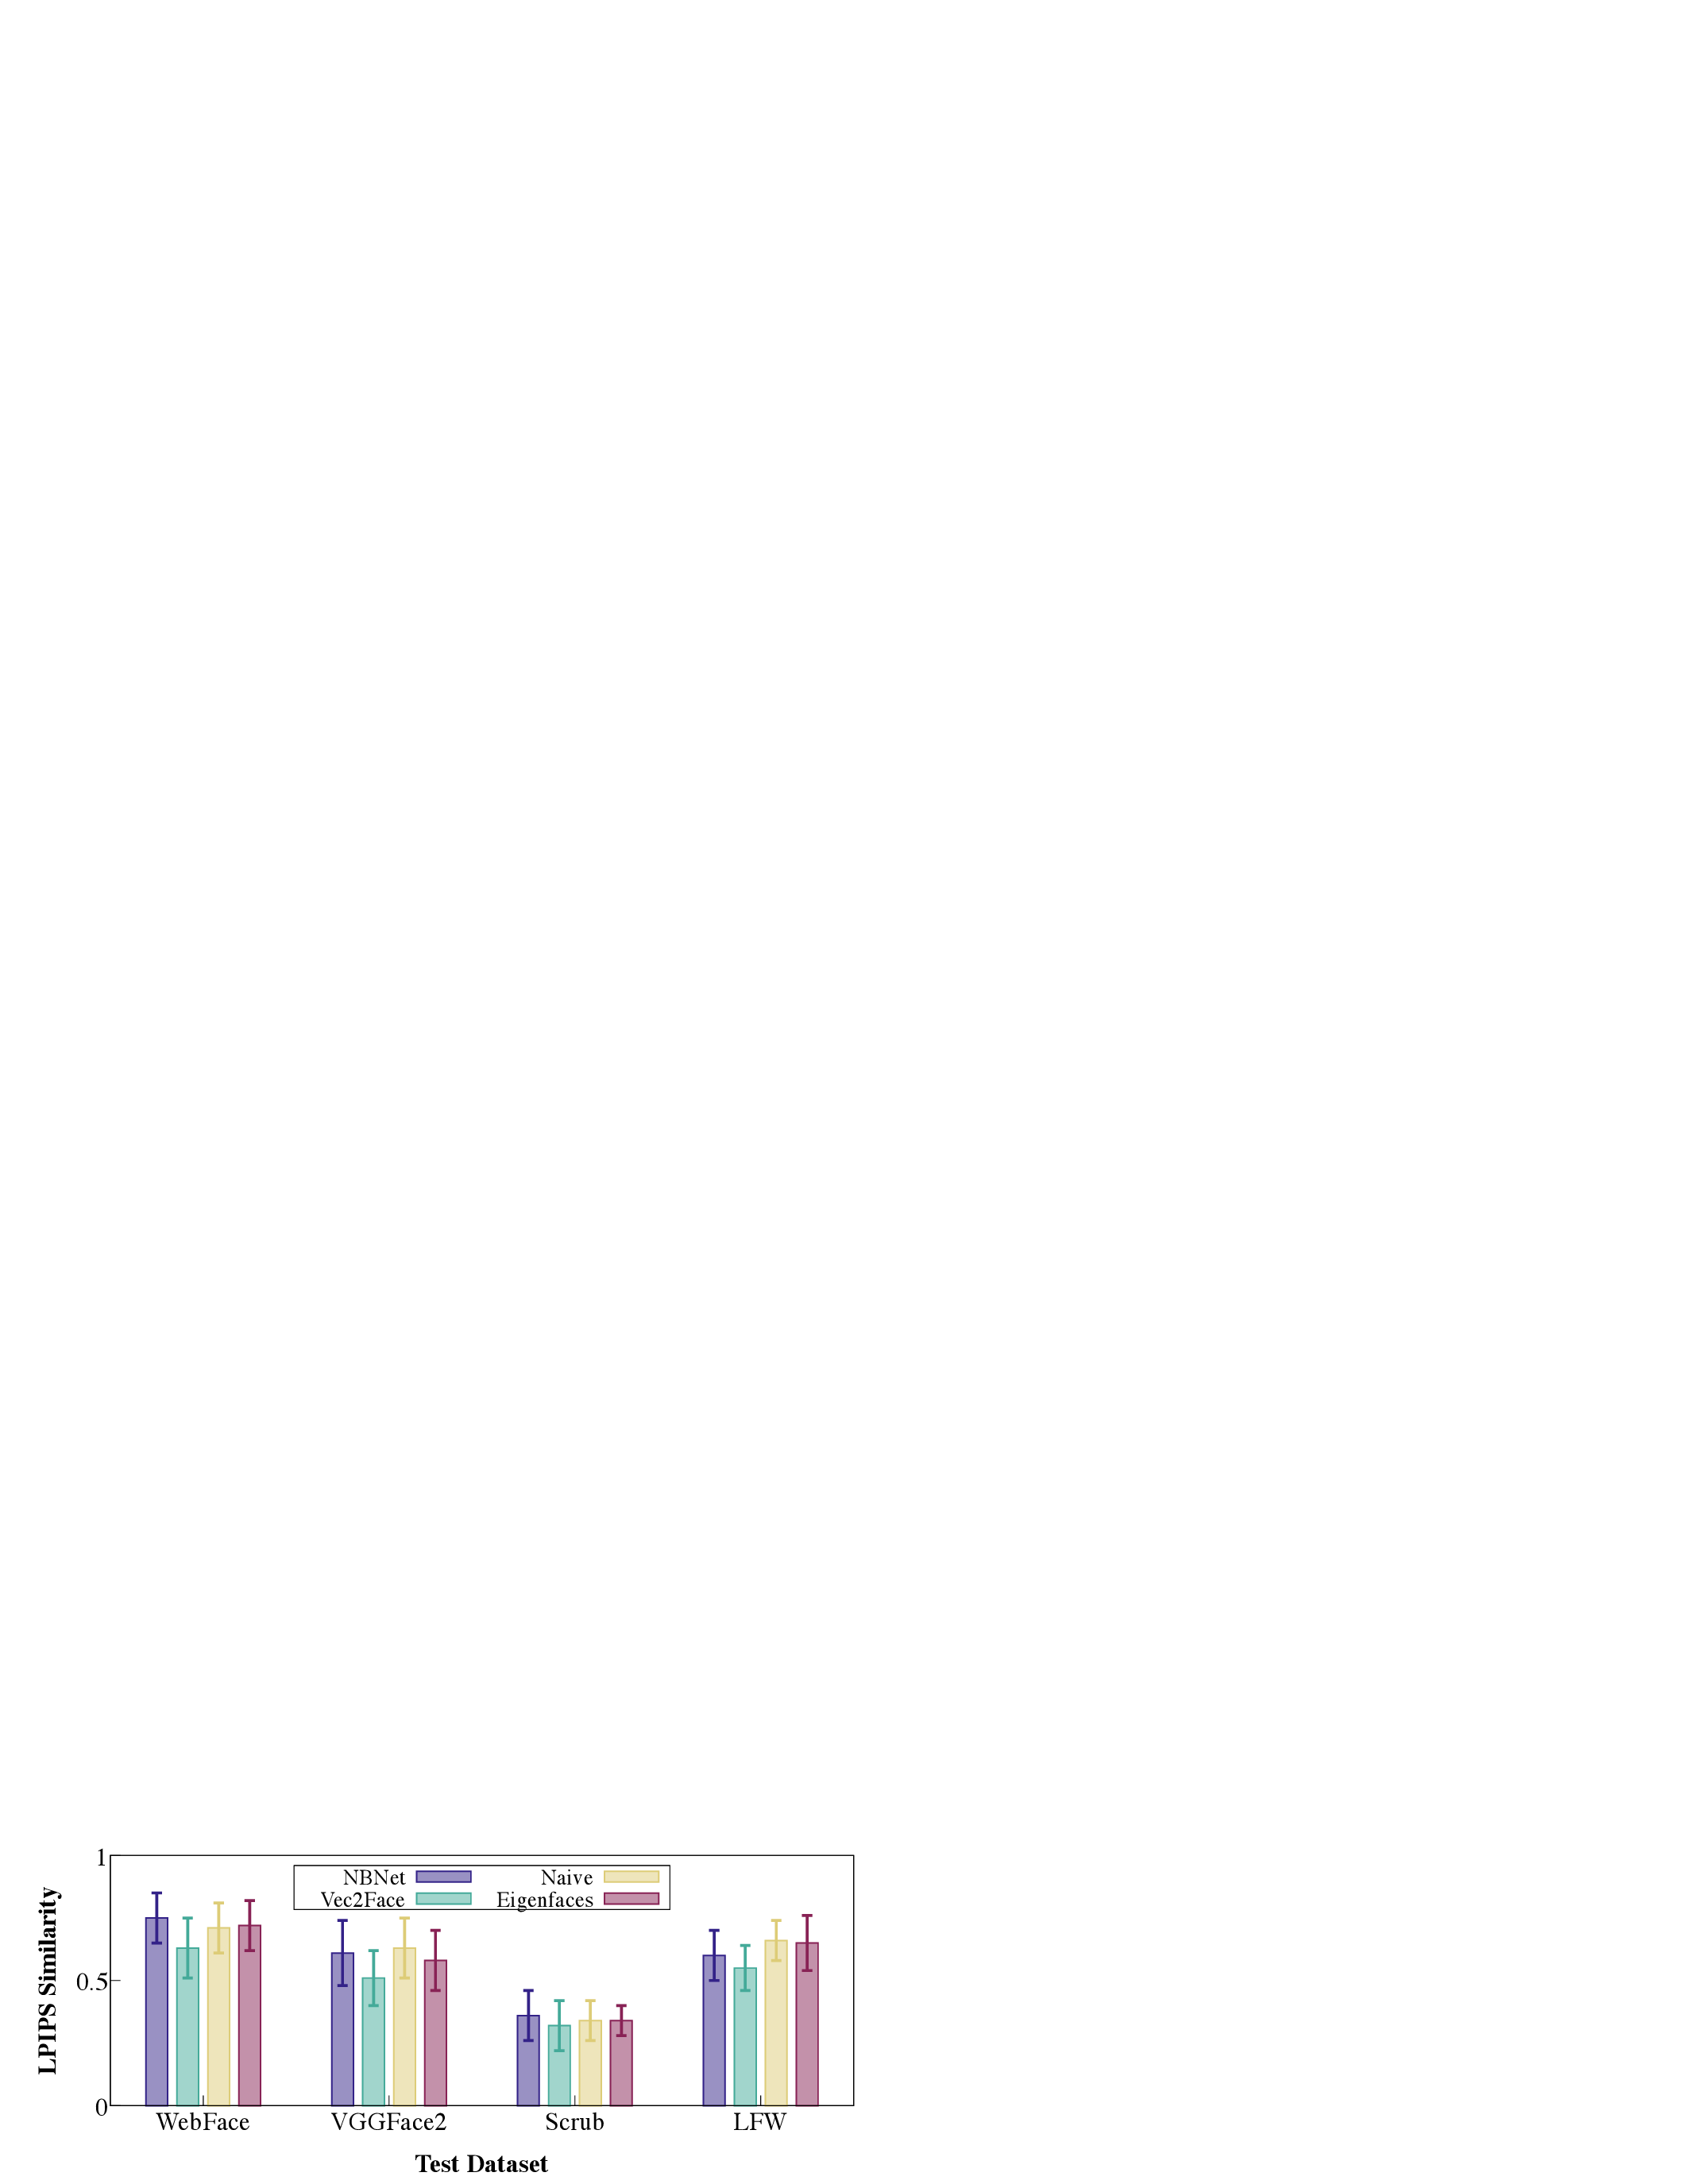}
  \captionof{figure}{\em Visual similarity between oariginal image and
    reconstruction across different datasets and reconstruction methods.}
  \label{fig:visual1}
\end{minipage}%
\hspace{0.2cm}
\begin{minipage}{.37\textwidth}
  \centering
  \includegraphics[width=.99\linewidth]{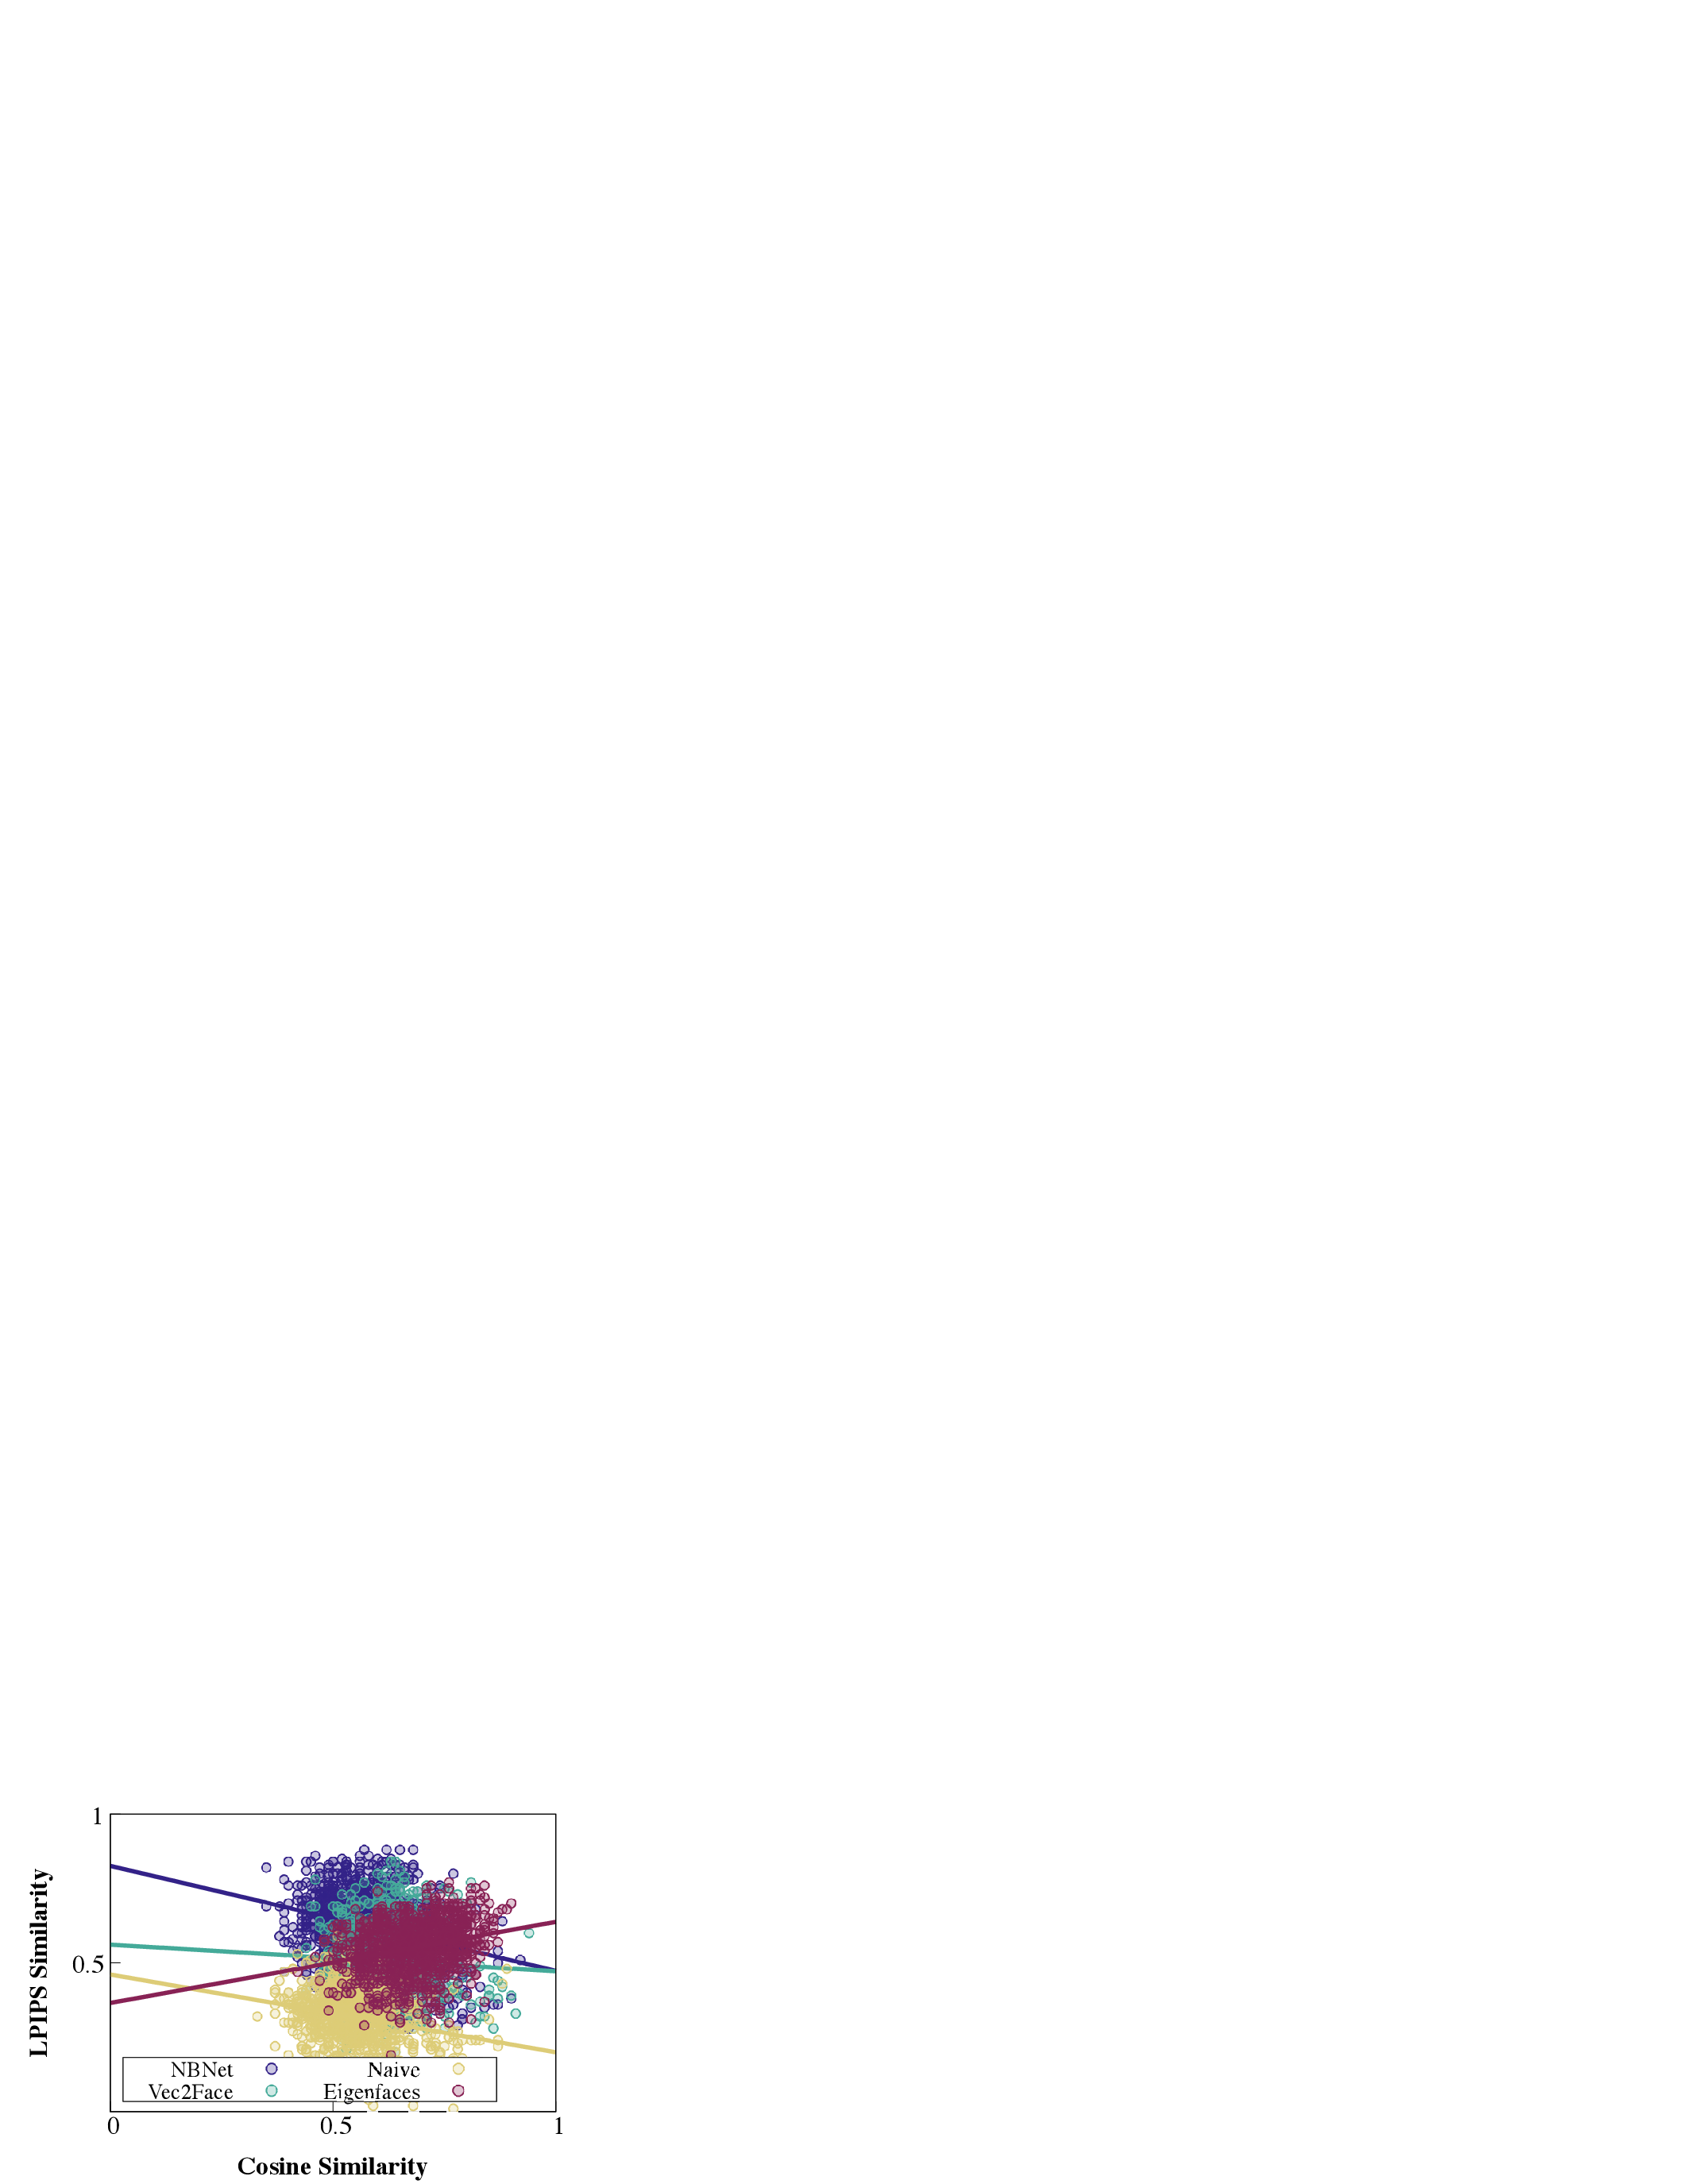}
  \captionof{figure}{{\em Feature space (x-axis) and visual similarity (y-axis) are not strongly correlated.}} %
  \label{fig:visual2}
\end{minipage}
\end{figure}
